# Supplementary material for: The origin of the high metallicity of close-in giant exoplanets II The nature of the sweet spot for accretion
Source: arXiv:2112.12623 source file (2021-12-23)
Supplement: Supplementary file 1 [file appendix_MMR.tex]

\section{Mean motion resonances and disturbing function}
We consider the motion of two particles with mass $m$ and $m^\prime$ orbiting around a central star with mass $m_{\rm c}$.
The orbital elements of the inner particle are given by $a$ (semi-major axis), $e$ (eccentricity), $i$ (inclination), $\Omega$ (longitude of ascending node), $\varpi$ (longitude of pericenter) and $\epsilon$ (mean longitude at epoch), respectively.
$\lambda$ is a mean longitude defined as 
\begin{align}
    \lambda=n t+\epsilon,
\end{align}
where $n$ is the mean motion.
The orbital parameters of the outer particle are denoted with prime.
When the mean motion of the inner particle has a simple relation with that of the outer particle, namely
\begin{align}
    \frac{n^\prime}{n} \sim \frac{p}{p+q},
\end{align}
where $p$ and $q$ are integers, the inner particle is in the $p+q:p$ mean motion resonance with the outer one.
In this case, the conjunction with the outer particle is limited at some fixed points on the orbit.
The accumulative gravitational perturbation from the outer particle deforms the orbit of the inner particle significantly.

To derive the change rates of orbital elements by mean motion resonances, we introduce the disturbing function $\mathcal{R}$ ($\mathcal{R}^\prime$), which is the potential of the inner (outer) particle associated with perturbation from the outer (inner) particle.
The disturbing function is given as \citep{Murray+1999}
\begin{align}
    \mathcal{R}             = \frac{\mathcal{G} m^\prime}{m_{\rm c}} \sum_{j_i} S \cos \varphi, \label{eq:disturbing_function_in} \\
    \mathcal{R}^{\prime}    = \frac{\mathcal{G} m       }{m_{\rm c}} \sum_{j_i} S \cos \varphi, \label{eq:disturbing_function_out}
\end{align}
where
\begin{align}
    S       &\approx \frac{f(\alpha)}{a^\prime} e^{|j_4|} {e^\prime}^{|j_3|} s^{|j_6|} {s^\prime}^{|j_5|}, \label{eq:disturbing_function_strength}
\end{align}
with $\mathcal{G}$ is a gravitational constant, $f(\alpha)$ is a function of Laplace coefficients \citep[see][]{Murray+1999}, $s=\sin 1/2 i$, $s^\prime=\sin 1/2 i^\prime$, and $\phi$ is an argument given by
\begin{align}
    \varphi &= j_{\rm 1} \lambda^{\prime} +j_{\rm 2} \lambda +j_{\rm 3} \varpi^{\prime} +j_{\rm 4} \varpi +j_{\rm 5} \Omega^{\prime} +j_{\rm 6} \Omega, \label{eq:resonant_argument}
\end{align}
with $j_i$ being integers that sustain the d'Alembert relation
\begin{align}
    \sum_{i=1}^6 j_i = 0. \label{eq:dAlembert_relation}
\end{align}
The function $S$ indicates the strength of each term of the disturbing function.
The disturbing function is given as an infinite series and each term contains $\cos \varphi$.
Outside the mean motion resonances, $\cos \varphi$ changes on the conjunction timescale because the argument $\varphi$ increases or decreases with time.
Inside the $p+q:p$ mean motion resonance, however, there is a resonant argument that barely changes with time because the time derivative of the resonant argument $\dot{\varphi}$ is given as
\begin{align}
    \dot{\varphi} &\sim (p+q) n^{\prime} -p n \sim 0. \label{eq:dot_resonant_argument_approximation}
\end{align}
In the long-term orbital evolution, integrated terms except the resonant terms of the disturbing function are almost zero.
Thus, the orbital evolution of particles in mean motion resonances are regulated by only a few resonant terms in the disturbing function.

Considering the long period orbital evolution of each particle, we integrate and average Lagrange's equations of motion below.
As discussed above, almost all terms except the resonant terms in the disturbing function are negligibly small.
In practice, we use the averaged disturbing function $\left< \mathcal{R} \right>$ and $\left< \mathcal{R}^\prime \right>$ given as
\begin{align}
    \left< \mathcal{R} \right> &= \frac{\mathcal{G} m^{\prime}}{a^{\prime}} \left[ \mathcal{R}_{\rm D}^{\rm (sec)} + e^{|j_{\rm 4}|} {e^{\prime}}^{|j_{\rm 3}|} s^{|j_{\rm 6}|} {s^{\prime}}^{|j_{\rm 5}|} \left\{ f_{\rm d}(\alpha) +f_{\rm e}(\alpha) \right\} \cos \varphi \right], \\
    \left< \mathcal{R}^{\prime} \right> &= \frac{\mathcal{G} m}{a} \left[ \alpha \mathcal{R}_{\rm D}^{\rm (sec)} + e^{|j_{\rm 4}|} {e^{\prime}}^{|j_{\rm 3}|} s^{|j_{\rm 6}|} {s^{\prime}}^{|j_{\rm 5}|} \left\{ \alpha f_{\rm d}(\alpha) +f_{\rm i}(\alpha) \right\} \cos \varphi \right],
\end{align}
where $\alpha=a/a^{\prime}$, $\mathcal{R}_{\rm D}^{\rm (sec)}$ is a secular term, and $f_{\rm d}$, $f_{\rm e}$ and $f_{\rm i}$ are a direct term, external indirect term and internal indirect term, respectively (see also below).
The equations of motion in orbital elements are called as Lagrange's equations and written with the disturbing function.
The Lagrange's equations in the lowest-order terms in terms of $e$ and $i$ are given by
\begin{align}
    \dot{a}         &=  \frac{2}{n a}           \frac{\partial \left< \mathcal{R} \right>}{\partial \lambda}, \\
    \dot{e}         &= -\frac{1}{n a^2 e}       \frac{\partial \left< \mathcal{R} \right>}{\partial \varpi}, \\
\end{align}

Hereafter, we consider a restricted three-body problem where the perturbing particle is much heavier than the perturbed particle ($m\ll~m^\prime$ or $m\gg~m^\prime$) and the former is in a circular orbit.
Both particles move on the reference plane.
This situation is close to the cases that we consider in the following chapters.
The averaged disturbing function is reduced to
\begin{align}
    \left< \mathcal{R}        \right> &= \frac{\mathcal{G}m^\prime}{a^\prime} \left[        f_{\rm s} (\alpha) e^2 +       f_{\rm d} (\alpha) e^{|j_4|} \cos \varphi          \right], \\
    \left< \mathcal{R}^\prime \right> &= \frac{\mathcal{G}m       }{a       } \left[ \alpha f_{\rm s} (\alpha) e^2 +\alpha f_{\rm d} (\alpha) e^{|j_3|} \cos \varphi^\prime   \right],
\end{align}
where $f_{\rm s}$ is a secular term coming from $\mathcal{R}_{\rm D}^{\rm (sec)}$.
The resonant arguments are  
\begin{align}
    \varphi        &= j_1 \lambda^\prime +j_2 \lambda +j_4 \varpi, \\
    \varphi^\prime &= j_1 \lambda^\prime +j_2 \lambda +j_3 \varpi^\prime.
\end{align}
We can reduce the above equations of motion for the inner particle into
\begin{align}
    \dot{n}         &= 3 j_{\rm 2} C_{\rm r} n e^{|j_{\rm 4}|}   \sin \varphi, \label{eq:Lagrange_axi_int} \\
    \dot{e}         &=   j_{\rm 4} C_{\rm r}   e^{|j_{\rm 4}|-1} \sin \varphi, \label{eq:Lagrange_ecc_int}
\end{align}
with
\begin{align}
    C_{\rm r} =\frac{m^{\prime}}{m_{\rm c}} n \alpha f_{\rm d} (\alpha), \label{eq:Lagrange_Cr_int}
\end{align}
and for the outer particle into
\begin{align}
    \dot{n^{\prime}} &= 3 j_{\rm 1} C_{\rm r}^{\prime} n^{\prime} {e^{\prime}}^{|j_{\rm 3}|}   \sin \varphi^\prime, \label{eq:Lagrange_axi_ext} \\
    \dot{e^{\prime}} &=   j_{\rm 3} C_{\rm r}^{\prime}            {e^{\prime}}^{|j_{\rm 3}|-1} \sin \varphi^\prime, \label{eq:Lagrange_ecc_ext}
\end{align}
with
\begin{align}
    C_{\rm r}^{\prime} =\frac{m}{m_{\rm c}} n^{\prime} f_{\rm d} (\alpha). \label{eq:Lagrange_Cr_ext}
\end{align}
Table \ref{tab:interaction_coefficient} gives the values of $f_{\rm s}$ and $f_{\rm d}$.

%%%%%%%%%%%%%%%%%%%%%%%%%%%%%%%%%%%%%%%%%%%%%%%%%%%%%%%%%%%%%
\begin{table}[t]
    \centering
    \begin{tabular}{c|c|c} \hline
        $p+q:p$ & $f_{\rm s}$ & $f_{\rm d}$  \\ \hline
        2:1     & $0.387627$ & $-1.19049$ \\
        3:2     & $1.15279$  & $-2.02521$ \\
        4:3     & $2.27923$  & $-2.84042$ \\
        5:4     & $3.76541$  & $-3.64962$ \\ \hline
    \end{tabular}
    \caption{Values of the secular term $f_{\rm s}$ and the direct term $f_{\rm d}$ for the first order mean motion resonances.}
    \label{tab:interaction_coefficient}
\end{table}
%%%%%%%%%%%%%%%%%%%%%%%%%%%%%%%%%%%%%%%%%%%%%%%%%%%%%%%%%%%%%

\subsection{Libration timescale and resonant width}\label{sec:pendulumn_model}
Inside the mean motion resonances, the resonant argument librates on a libration timescale $\tau_{\rm lib}$.
Along with the libration of the resonant argument, the semi-major axis of the inner and outer particle also librate and the maximum change in the semi-major axis $\delta a_{\rm max}$ and $\delta a_{\rm max}^{\prime}$ can be written as \citep{Murray+1999}

\begin{align}
    \frac{\delta a_{\rm max,\pm}}{a} &= \pm \left( \frac{16}{3} \frac{|C_{\rm r}|}{n} e \right)^{1/2} \left( 1+\frac{1}{27 {j_{\rm 2}}^2 e^3} \frac{|C_{\rm r}|}{n}\right)^{1/2} - \frac{2}{9 j_{\rm 2} e} \frac{|C_{\rm r}|}{n}, \label{eq:1st_order_resonant_width_in} \\
    \frac{\delta {a^{\prime}}_{\rm max,\pm}}{a^{\prime}} &= \pm \left( \frac{16}{3} \frac{|C_{\rm r}^{\prime}|}{n^{\prime}} e^{\prime} \right)^{1/2} \left( 1+\frac{1}{27 {j_{\rm 1}}^2 {e^{\prime}}^3} \frac{|C_{\rm r}^{\prime}|}{n^{\prime}}\right)^{1/2} - \frac{2}{9 j_{\rm 1} e^{\prime}} \frac{|C_{\rm r}^{\prime}|}{n^{\prime}} \label{eq:1st_order_resonant_width_out}.
\end{align}
%The libration timescale of internal and external resonances are \citep{Murray+1999}
%\begin{align}
%    \tau_{\rm lib} &= \frac{2 \pi}{n} \left| \left|\frac{j_2}{j_1} \right|^{4/3} \left( \frac{m^{\prime}}{m_c} \right)^2 \frac{{f_{\rm d}}^2 (\alpha)}{e^2}
%                        - 3 {j_2}^2 \left|\frac{j_2}{j_1} \right|^{2/3} \frac{m^{\prime}}{m_c} f_{\rm d} (\alpha) e \right|^{-1/2}, \label{eq:1st_order_libration_time_in} \\
%    \tau_{\rm lib}^{\prime} &= \frac{2 \pi}{n^{\prime}} \left| \left( \frac{m}{m_c} \right)^2 \frac{{f_{\rm d}}^2 (\alpha)}{{e^{\prime}}^2}
%                        - 3 {j_1}^2 \frac{m}{m_c} f_{\rm d} (\alpha) e^{\prime} \right|^{-1/2}. \label{eq:1st_order_libration_time_out}
%\end{align}
%Figure~\ref{fig:Review_resonances} shows the locations of the three first-order inner mean motion resonances with a Jupiter-mass planet orbiting at $5\AU$ in the $a$-$e$ plane.
%Inside the color-coded regions, the resonant arguments librate on a timescale of $\tau_{\rm lib}$ and the semi-major axis and eccentricity of the perturbed particle evolve according to eq.~(\ref{eq:Lagrange_axi_int}) and eq.~(\ref{eq:Lagrange_ecc_int}).
%The width of the resonance is defined as
%\begin{align}
%    \Delta a_{\rm res} = \left| \delta a_{\rm max,+}-\delta a_{\rm max,-} \right|, \label{eq:1st_order_resonant_width}
%\end{align}
%
%and takes the minimum value at
%\begin{align}
%    e = \frac{2^{1/3}}{3} \left( \left|j_1\right|^{-2/3} \left|j_2\right|^{-4/3} f_{\rm d} \frac{m}{m_{\rm c}} \right)^{1/3}. \label{eq:ecc_at_minimum_resonant_width}
%\end{align}

%%%%%%%%%%%%%%%%%%%%%%%%%%%%%%%%%%%%%%%%%%%%%%%%%%%%%%%%%%%%%
\begin{figure}
  \begin{center}
    \includegraphics[width=80mm]{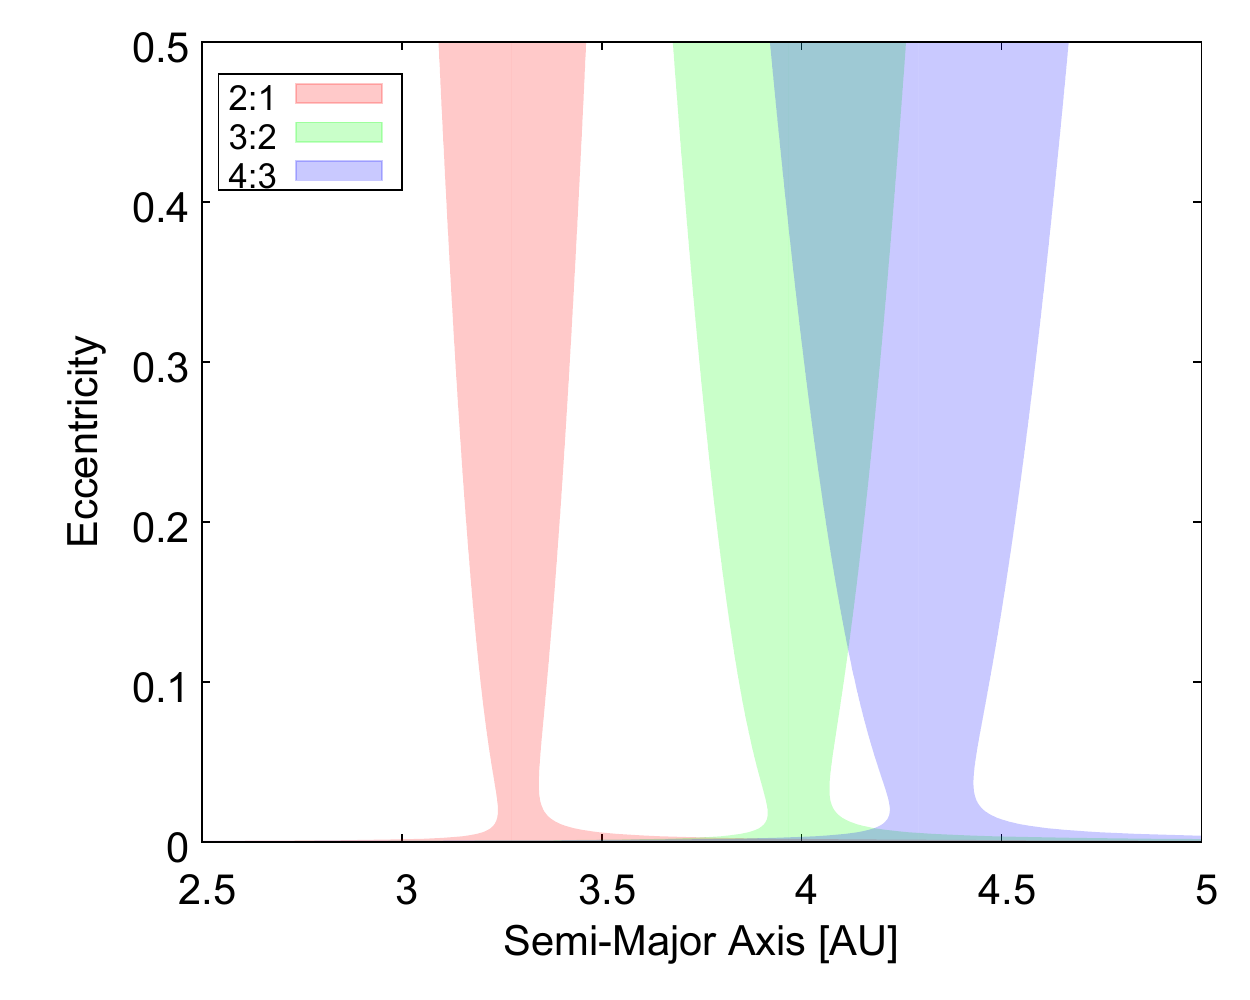}
    \caption{
    The locations of the first-order mean motion resonances with a Jupiter-mass planet at $5 \AU$ in the $a$-$e$ plane.
    Here, we show the $2:1$ (red), $3:2$ (green) and $4:3$ (blue) resonances.
    }
    \label{fig:Review_resonances}
  \end{center}
\end{figure}
%%%%%%%%%%%%%%%%%%%%%%%%%%%%%%%%%%%%%%%%%%%%%%%%%%%%%%%%%%%%%
