# Supplementary material for: The origin of the high metallicity of close-in giant exoplanets II The nature of the sweet spot for accretion
Source: arXiv:2112.12623 source file (2021-12-23)
Supplement: Supplementary file 2 [file appendix_Model.tex]

In sec.~\ref{sec:sweet_spot_compare}, we performed N-body simulations and compare the results with the analytical expressions for the sweet spot.
The model we used depends on that in \citet{Shibata+2020}.
Here summarise the model briefly.

In our model, we assume the following situation: 
a giant planet has finished gas accretion and the planet is no longer growing in mass. 
The planet then migrates radially inward from a given semi-major axis in a circumstellar disk.
Initially there are many single-sized planetesimals interior to the planet's orbit.  
The migrating planet then encounters these planetesimals and captures some of them. 
The planetesimals are represented by test particles and, therefore are affected only by the gravitational forces from the central star and planet, and the drag force by the disk gas.
The dynamical integration for these bodies is performed using the numerical simulation code developed in \citet{Shibata+2019}.
In the code, we integrate the equation of motion using the forth-order-Hermite integration scheme \citep{Makino+1992}.
For timestep, we adopt the method of \citep{Aarseth1985}.

\subsection{Equations of motion}\label{sec:app_eom}
The equation of motion is given by
\begin{align}
   \frac{{\rm d} {\bf r}_{\rm i} }{{\rm d} t} &= \sum_{i\neq j} {\bf f}_{{\rm grav},i,j} + {\bf f}_{\rm aero} +{\bf f}_{\rm tide}, \label{eq:EoM}
\end{align}
where ${\bf r}_i$ is the position vector relative to the initial (i.e., $t = 0$) mass centre of the star-planet-planetesimals system, %$t$ is the time, 
${\bf f}_{{\rm grav},i,j}$ is the mutual gravity between particles $i$ and $j$ given by
\begin{align}
   {\bf f}_{{\rm grav},i,j} &= - \mathcal{G} \frac{M_{\rm j}}{{r_{i,j}}^3} {\bf r}_{i,j} \label{eq:EoM_gravity}
\end{align}
with $\mathbf{r}_{i,j}$ being the position vector of particle $i$ relative to particle $j$ ($r_{i,j} \equiv |{\bf r}_{i,j}|$),
$M_{\rm j}$ is the mass of particle $j$, and $\mathcal{G}$ is the gravitational constant,
${\bf f}_{\rm aero}$ is the aerodynamic gas drag, and ${\bf f}_{\rm tide}$ is the gravitational tidal drag from the circumstellar disk gas. 
The central star, planet, and planetesimals are denoted by the subscripts $i$ (or $j$) = 1, 2, and $\geq$~3, respectively.
The planetesimals are treated as test particles; therefore $f_{{\rm grav},i,j}=0$ in Eq.~(\ref{eq:EoM}) for $j \geq~3$.
The aerodynamic gas drag force \citep{Adachi+1976} and the tidal drag force are given by
\begin{align}
  {\bf f}_{\rm aero} &= -\frac{{\bf u}}{\tau_{\rm aero}}. \label{eq:EoM_reduced_gas_drag} \\
  {\bf f}_{\rm tide} &= - \frac{{\bf v}_{\rm p}}{2 \tau_{{\rm tide},a}},
\end{align}
with
\begin{align}
    \tau_{\rm aero} &=  - \frac{2 m_{\rm pl}}{ C_{\rm d} \pi R_{\rm pl}^2 \rho_{\rm gas} u} \\
    \tau_{{\rm tide},a} &= \tau_{\rm tide,0} \left( \frac{a_{\rm p}}{1 \AU} \right)^{1/2}, \label{eq:type2_migration_timescale}
\end{align}
Here ${\bf u}={\bf v}_{\rm pl}-{\bf v}_{\rm gas}$ ($u = |{\bf u}|$) is the planetesimal velocity (${\bf v}_{\rm pl}$) relative to the ambient gas (${\bf v}_{\rm gas}$), %$\tau_{\rm aero}$ is the timescale of aerodynamic gas drag, 
$m_{\rm pl}$ is the planetesimal's mass, 
$C_{\rm d}$ is the non-dimensional drag coefficient and given as $C_{\rm d}=1$, 
$\rho_{\rm gas}$ is the gas density,
$R_{\rm pl}$ is the planetesimal's radius,
${\bf v}_{\rm p}$ is the planet's velocity,
$a_{\rm p}$ is the planet's semi-major axis,
and $\tau_{\rm tide,0}$ is a scaling parameter.
The velocity and density of the ambient disk gas are calculated from the circumstellar disk model.
Given the range of the planetesimal mass ($\sim10^{16}$-$10^{22} \g$) and planet ($\sim10^{30} \g$), we assume $f_{\rm tide}=0$ for the former and $f_{\rm aero}=0$ for the latter.
The central star is not affected by $f_{\rm aero}$ and $f_{\rm tide}$.

%In type II regime, the dependence on ${a_{\rm p}}$ changes with the condition of surrounding disk gas and $\tau_{\rm tide,0}$ depends on the planetary mass and the disk profiles around the planet \citep[e.g.][]{Lin+1993,Kanagawa+2018}.
%However, we fix the exponent of ${a_{\rm p}}$ as $1/2$, which is the limiting case where the planet mass is heavier than the surrounding disk gas, and $\tau_{\rm tide,0}$ as constant in our simulation.
%This simplification allows a systematic investigation of the effect of planet migration on the efficiency of planetesimal accretion.

\subsection{Disk model}\label{sec:app_disk}
We adopt the minimum-mass solar nebula model \citep{Hayashi1981} as our gas disk model.
The surface density $\Sigma_{\rm gas}$ is expressed as
\begin{align}\label{eq:Disk_Gas_MMSN}
    \Sigma_{\rm gas} = \Sigma_{\rm gas,0} \left( \frac{r}{1\AU} \right)^{-\alpha_{\rm disk}},
\end{align}
where $r$ is a radial distance from initial mass centre of the star-planet system, $\Sigma_{\rm gas,0} = 1.7 \times 10^3 \g/\cm^3$ and $\alpha_{\rm disk}=3/2$.
The temperature of the circumstellar disk $T_{\rm disk}$ is given by: 
\begin{align}
    T_{\rm disk} = T_{\rm disk,0} \left(\frac{r}{1\AU} \right)^{-2\beta_{\rm disk}},
\end{align}
where $T_{\rm disk,0}=280~\K$ and $\beta_{\rm disk}=1/4$.
The circumstellar disk being assumed to be vertically isothermal, the gas density $\rho_{\rm gas}$ is expressed as
\begin{align}\label{eq:Disk_Gas_volume}
   \rho_{\rm gas} = \frac{\Sigma_{\rm gas}}{\sqrt{2 \pi} h_{\rm s}} \exp \left( -\frac{z^2}{2 {h_{\rm s}}^2} \right),
\end{align}
where $z$ is the height from the disc mid-plane and $h_{\rm s}$ is the disk's scale height.
The aspect ratio of the circumstellar disk is 
\begin{align}
    \frac{h_{\rm s}}{r} = \frac{c_{\rm s}}{r\Omega_{\rm K}},
\end{align}
where $\Omega_{\rm K}$ is a Kepler angular velocity and $c_{\rm s}$ is a sound speed of disk gas.
The sound speed is given as %Assuming locally isothermal case, 
\begin{align}
    c_{\rm s} = \sqrt{\frac{k_{\rm B} T_{\rm disk}}{\mu_{\rm disk} m_{\rm H}}} \propto r^{-\beta{\rm disk}},
\end{align}
where $k_{\rm B}$ is the Boltzmann constant and $\mu_{\rm disk}$ is a mean molecular weight in a unit of proton mass $m_{\rm H}$.
In this study, $\mu_{\rm disk}$ is set as $2.3$ and the aspect ratio of the disk gas at $1\AU$ is $\sim0.03$.

The gas in the circumstellar disk rotates with a sub-Keplerian velocity because of pressure gradient; namely
\begin{align}\label{eq:Disk_Gas_Velocity_sub-Kepler}
	v_{\rm gas} = v_{\rm K} \left( 1-\eta_{\rm disk} \right)
\end{align}
with $\eta_{\rm disk}$ defined as
\begin{align}
	\eta_{\rm gas} &\equiv	\mathbf{-} \frac{1}{2} \left( \frac{h_{\rm s}}{r} \right)^2 \frac{{\rm d} \ln P_{\rm gas}}{{\rm d} \ln r}, \label{eq:eta_gas_definition} \\ 
	               &=		\frac{1}{2} \left( \frac{h_{\rm s}}{r} \right)^2 
	                        \left[ \frac{3}{2} \left( 1 - \frac{z^2}{{h_{\rm s}}^2} \right) +\alpha_{\rm disk} +\beta_{\rm disk} \left(1+\frac{z^2}{{h_{\rm s}}^2}  \right) \right],
\end{align}
where $P_{\rm gas}$ is the gas pressure.
For deriving the above equation, we assume $\eta_{\rm gas} \ll 1$ and use the ideal-gas relation for isothermal sound speed, i.e., $c_{\rm s}^2$ = $P_{\rm gas} / \rho_{\rm gas}$.


We adopt a simple disk model for the solid surface density $\Sigma_{\rm solid}$, which is expressed as
\begin{align}
    \Sigma_{\rm solid} = \Sigma_{\rm solid,0} \left( \frac{r}{1\AU} \right)^{-\alpha_{\rm disk}^{\prime}} \label{eq:Model_Disk_Solid_Surface_Density}
\end{align}
In our model, we set $\alpha_{\rm disk}^{\prime}=\alpha_{\rm disk}=3/2$ and 
\begin{align}
    \Sigma_{\rm solid,0} = Z_{\rm s} \Sigma_{\rm gas,0},    
\end{align}
where $Z_{\rm s}$ is the solid-to-gas ratio, which is assumed equal to the metallicity of the central star.
The planetesimal's mass $m_{\rm pl}$ is calculated as $4\pi\rho_{\rm pl}{R_{\rm pl}}^3/3$, where $\rho_{\rm pl}$ is the planetesimal's mean density.
The surface number density of planetesimals is given as $\Sigma_{\rm solid}/m_{\rm pl}$ which gives $\sim10^6~/\AU^2$ at maximum.
To speed up the numerical integration, we adapt super-particles, which represent the orbits of several planetesimals, for the integration of planetesimal orbits.

We follow the orbital motion of super-particles, each of which contains several equal-size planetesimals.
The super-particles are distributed in a given radial region, where the inner and outer edges are denoted by $a_{\rm pl,in}$ and $a_{\rm pl,out}$, respectively. 
The surface number density of super-particles $n_{\rm s}$ is given as% $\propto r^{-3/2}$. 
\begin{align}
    n_{\rm s} = n_{\rm s,0} \left( \frac{r}{1 \AU} \right)^{-\alpha_{\rm sp}}
\end{align}
where
\begin{align}
    n_{\rm s,0} = \frac{N_{\rm sp}}{2 \pi} \frac{2 -\alpha_{\rm sp}}
                  {\left(a_{\rm pl,out}/1\AU\right)^{2-\alpha_{\rm sp}} -\left(a_{\rm pl,in}/1\AU\right)^{2-\alpha_{\rm sp}} } \left[\frac{1}{\AU^2}\right].
\end{align}
$N_{\rm sp}$ is the number of super-particles used in a given simulation.
In our simulation, we set $N_{\rm sp}=12,000$ and $\alpha_{\rm sp}=1$, which distribute super-particles uniformly in radial direction.
The mass per super-particle $M_{\rm sp}$ is given by
\begin{align}
    M_{\rm sp} (a_{\rm 0}) = \frac{\Sigma_{\rm solid} (a_{\rm 0})}{n_{\rm s} (a_{\rm 0})} ,
\end{align}
where $a_{\rm 0}$ is the initial semi-major axis of the super-particle.

As for eccentricity and inclination, assuming that planetesimals are scattered by their mutual gravitational interaction, we adopt the Rayleigh distribution as the initial eccentricities $e$ and inclinations $i$ of planetesimals.
We set $\left< e \right>^{1/2}=2\left< i \right>^{1/2}=10^{-3}$.
The orbital angles $\Omega$, $\varpi$ and $\epsilon$ are distributed uniformly.

During the orbital integration, we judge that a super-particle has been captured by the planet once (i) the super-particle enters the planet's envelope or (ii) its Jacobi energy becomes negative in the Hill sphere.
The planet's radius $R_{\rm p}$ is calculated as
\begin{align}\label{eq:Rplanet_cap}
    R_{\rm p} = \left( \frac{3 M_{\rm p}}{4 \pi \rho_{\rm p}} \right)^{1/3},
\end{align}
where $\rho_{\rm p}$ is the planet's mean density.
We consider that the planet radius is still expanded because of the rapid gas accretion before planetary migration.
We set $\rho_{\rm p}=0.125~\g~\cm^{-3}$, which gives two times expanded planetary radius for Jupiter-mass planet relative to the current Jupiter radius.


%%%%%%%%%%%%%%%%%%%%%%%%%%%%%%%%%%%%%%%%%%%%%%%%%%%%%%%%%%%%%%%%%%%%%%%%%
%%%         Parameters                                                %%%
%%%%%%%%%%%%%%%%%%%%%%%%%%%%%%%%%%%%%%%%%%%%%%%%%%%%%%%%%%%%%%%%%%%%%%%%%
\subsection{Model settings}\label{sec:app_settings}
The planetesimals are initially distributed in $a_{\rm pl,in}< r < a_{\rm pl,out}$ and $a_{\rm pl,in}$ is fixed at $0.3 \AU$ in our simulation.
The planet is initially located in such a way that the inner boundary of the feeding zone is consistent with the outer edge of the planetesimals disk, namely 
\begin{align}
    a_{\rm p,0} = \frac{a_{\rm pl,out}}{1-2\sqrt{3} h}. \label{eq:part1_initial_semimajoraxis_planet}
\end{align}
The calculation is artificially stopped once the planet reaches the orbit of $a_{\rm p,f}=0.5 \AU$.
We investigate the planetesimal accretion in the reference case, where $\tau_{{\rm tide},0}=10^5~\yr$, $R_{\rm pl}=10^7~\cm$, $a_{\rm pl,out}=20~\AU$ and $M_{\rm p}=10^{-3}M_{\rm s}$.
In the reference case, the total amount of planetesimals are $M_{\rm tot} \sim 43 \Mear$.
The choices of the parameter values for the reference model are summarised in Table~\ref{tb:settings}.
We perform a parameter study for different values of  $\tau_{\rm tide,0}$, $R_{\rm pl}$, and $M_{\rm p}$.% and investigate their effects on the captured heavy-element mass.

%Again, in this study, to focus on the effect of planetary migration on the planetesimal accretion, we do not consider planetary growth nor disk evolution. 
%While our setup is simplified, it allows us to identify the parameters that strongly influence the planetesimals orbital evolution and the efficiency of planetesimal accretion.
%This is discussed in detail.

\begin{table*}
	\centering
	\begin{tabular}{ llllll } % four columns, alignment for each
		%\hline
		%Parameters used in the model &&&&&\\
		\hline
		$M_{\rm s}$             & Mass of central star	                        & $1.0$				                & $\Msun$ 	\\
		$Z_{\rm s}$             & Metallicity of central star	                & $0.018$				            & - \\
		$M_{\rm p}$             & Mass of planet		                        & $1.0$		                        & $\Mjup$  \\
		$R_{\rm p}$             & Radius of planet		                        & eq.~(\ref{eq:Rplanet_cap})        & \\
		$\rho_{\rm p}$          & Mean density of planet                        & $0.125$                           & $\g~\cm^{-3}$ \\
        $a_{\rm p,0}$           & Initial semi-major axis of planet             & eq.~(\ref{eq:part1_initial_semimajoraxis_planet})  & \\
        $a_{\rm p,f}$           & Final semi-major axis of planet               & $0.5$                             & $\AU$ \\
		$\tau_{\rm tide,0}$     & Scaling factor of migration timescale	        & $1.0 \times 10^5$                 & $\yr$ \\
        $\Sigma_{\rm disk,0}$   & Surface density of disk gas at $1\AU$         & $1.7\times10^{3}$		            & $\g/\cm^2$  \\
        $T_{\rm disk,0}$        & Temperature at $1\AU$                         & $280$		                        & $\K$  \\
        $\alpha_{\rm disk}$     & Exponent of disk gas profile                  & $3/2$                             & - \\
        $\beta_{\rm disk}$      & Exponent of disk temperature profile          & $1/2$                             & - \\
        $R_{\rm pl}$            & Radius of planetesimal			            & $1.0 \times 10^6$	                & $\cm$		    \\
        $a_{\rm pl,in}$         & Inner edge of planetesimal disk	            & $0.3$	                            & $\AU$		    \\
        $a_{\rm pl,out}$        & Outer edge of planetesimal disk	            & $20$	                            & $\AU$		    \\
        $\alpha_{\rm sp}$       & Exponent of test particle distribution        & $1$                               & - \\
		$\rho_{\rm pl}$         & Mean density of planetesimal			        & $2.0$	                            & $\g~\cm^{-3}$		    \\
		$N_{\rm sp}$            & Initial number of super-particles             & 12 000                            & - \\
		\hline
	\end{tabular}
	\caption{
	Parameters used in the reference model.
    }
    \label{tb:settings}
\end{table*}
